# Supplementary material for: Magnetic-field dependence of spin-phonon relaxation and dephasing due to g-factor fluctuations from first principles
Source: arXiv:2411.18608 source file (2025-03-06)
Supplement: Supplementary file 1 [file supplementary-information.pdf]

# Supplementary Information for "Magnetic-field dependence of spin-phonon relaxation and dephasing due to $g$-factor fluctuations from first principles"

Joshua Quinton,[1] Mayada Fadel,[2] Junqing Xu,[3] Adela Habib,[4] Christian Multunas,[2] Mani Chandra,[2] Yuan Ping,[3,*] and Ravishankar Sundararaman[2,†]

[1]*Department of Physics, Applied Physics, and Astronomy, Rensselaer Polytechnic Institute, Troy, New York 12180, USA*
[2]*Department of Materials Science and Engineering, Rensselaer Polytechnic Institute, Troy, New York 12180, USA*
[3]*Department of Chemistry and Biochemistry, University of California, Santa Cruz, CA 95064, USA*
[4]*Theoretical Division, Los Alamos National Laboratory, Los Alamos, NM 87545, USA*
(Dated: February 10, 2025)

## I. DFT CALCULATION DETAILS AND CONVERGENCE

For each material shown, we performed *ab initio* electronic structure, Wannier function and phonon calculations using JDFTx, with norm-conserving pseudopotentials and the PBE exchange-correlation functional [1–3]. Figure 1 shows the DFT band structure compared to the Wannier interpolation for $CsPbBr_3$ and Si, while Figure 2 shows the corresponding phonon dispersions. Finally, Figure 3 shows that the electron, phonon and electron-phonon properties are all adequately converged with respect to $k$-points/supercell for accurate interpolation.

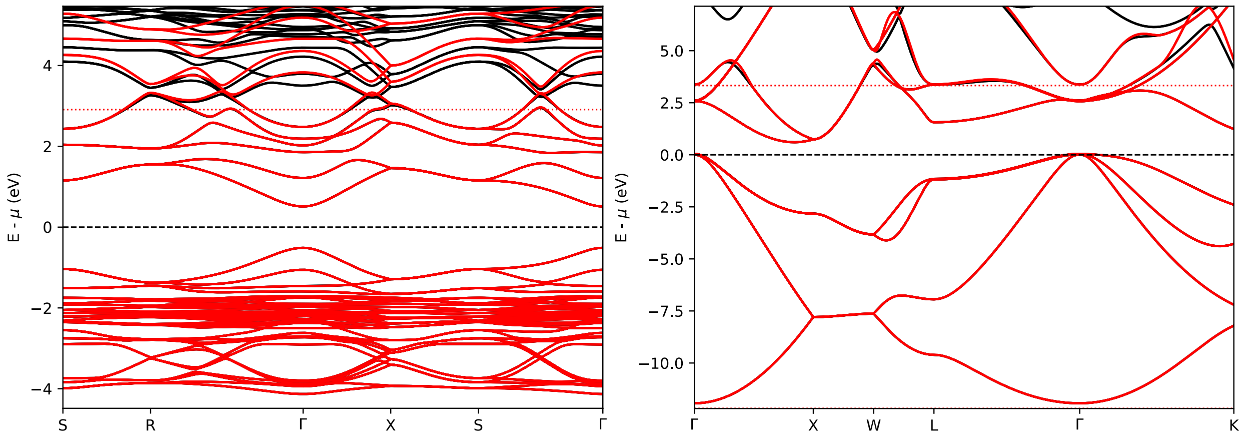


FIG. 1. Electronic band-structure of $CsPbBr_3$ (left) and Si (right), with excellent agreement between DFT (black) and Wannier interpolation (red); the axis range is restricted to the outer energy window and the red dotted line indicates the upper limit of the inner energy window.

## II. WANNIER AND DFT PHASE / UNITARY ROTATION MATCHING

To replace the Wannier matrix elements with DFT, we establish a workflow that ensures proper phase matching between them by comparing the momentum **P** and the spin **S** matrix elements, and then apply them to transform all the DFT matrix elements including the angular momentum **L** to the Wannier phase

* yuanping@ucsc.edu
† sundar@rpi.edu

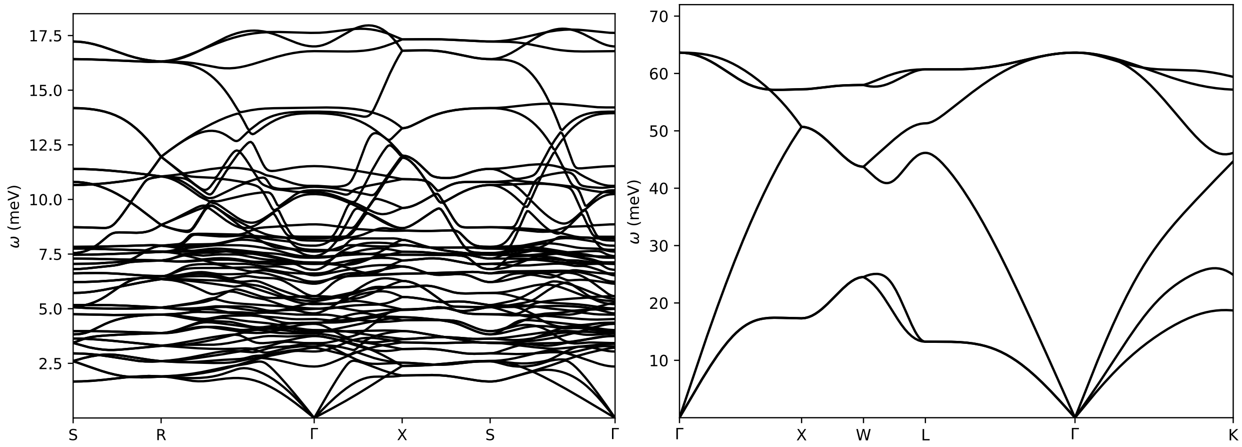


FIG. 2. Calculated phonon dispersions for $CsPbBr_3$ (left) and Si (right).

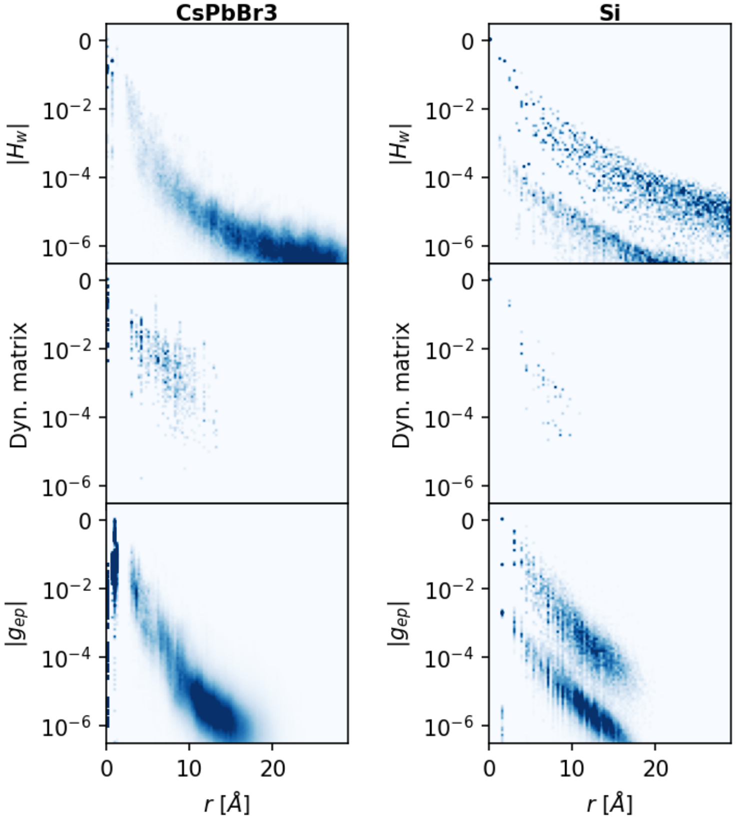


FIG. 3. The matrix elements of the Wannier Hamiltonian (top), dynamical matrix (middle) and electron-phonon coupling (bottom) all fall off exponentially with the distance between the Wannier centers and/or atoms for both $CsPbBr_3$ (left panels) and Si (right panels), indicating adequate $k$-point/supercell convergence of the electron, phonon and electron-phonon properties.

/ unitary rotations. There is an undetermined basis choice within each degenerate subspace, so we need to match these rotations between the different operators. So before applying the phase matching, unitary rotations are needed to have the same eigen-basis within each degenerate subspace.

For each degenerate subspace, we break the degeneracies of $\mathbf{P}$ and $\mathbf{S}$ with a perturbation Hamiltonian in

the subspace,

$$H^{dft} = \frac{\sum_{i=1}^{3}(a_i P_i^{dft} + b_i S_i^{dft})}{\sqrt{\sum_{i=1}^{3} a_i^2 + \sum_{i=1}^{3} b_i^2}} \tag{1}$$

$$H^{w} = \frac{\sum_{i=1}^{3}(a_i P_i^{w} + b_i S_i^{w})}{\sqrt{\sum_{i=1}^{3} a_i^2 + \sum_{i=1}^{3} b_i^2}} \tag{2}$$

where $i$ labels the 3 Cartesian components of $\mathbf{P}$ and $\mathbf{S}$. We repeat the above for randomly chosen $a_i$ and $b_i$ a number of times (for example 10) in order to select a perturbation that best resolves the degeneracies and thereby avoid accidental degeneracies that may still persist if we only used a specific component. For the case with best degeneracy resolution, we obtain the eigenvectors $V^{dft}$ and $V^w$ of $H^{dft}$ and $H^w$ respectively. $V^{dft}$ and $V^w$ then contain the unitary rotations needed to align the eigen-basis within this subspace.

After matching the degenerate-subspace rotations, we still have an undetermined phase $\phi_n$ for band $n$ between the Wannier and DFT. This leads to a phase difference between the off-diagonal elements of any operator between Wannier and DFT, for example $P^w_{i,mn} = e^{i(\phi_n - \phi_m)} P^{i,dft}_{mn}$. We extract the phases from

$$e^{i(\phi_n - \phi_m)} = \arg \sum_{i=1}^{3} \left( S^{dft*}_{i,mn} S^{w}_{i,mn} + P^{dft*}_{i,mn} P^{w}_{i,mn} \right) \tag{3}$$

which allows us to use the largest matrix elements available for each band pair to obtain the unknown phases in the most numerically stable way. After computing the unitary rotations within degenerate subspaces and the overall phases, we apply them to transform all the DFT matrix elements including the angular momentum $\mathbf{L}$ to the Wannier phases and degenarate subspace rotations.

## III. ANALYTICAL MODEL FOR SPIN RELAXATION DUE TO $g$-TENSOR FLUCTUATIONS

With an applied magnetic field $\mathbf{B}$, the Larmor precession of spins in a material with tensorial $g$-factors is given by $\mathbf{\Omega} = g \cdot \mu_B \mathbf{B}/\hbar$, where the magnitude of $\mathbf{\Omega}$ is the precession frequency and the direction is the axis of precession. Here, we derive a model for spin relaxation times that account for the fluctuation of both the frequency and the axis, and show in the main text that this accounts very well for the magnetic dependence of spin relaxation times ($T_1$, $T_2$ and $T_2^*$) fo $CsPbBr_3$ and Si.

Without loss of generality, let $\mathbf{B} \parallel \hat{z}$. Assuming that the off-diagonal components of $g$ are small compared to the diagonal part, the precession frequency $\Omega = \Omega_z + O(\Omega_{xy}^2)$ and $\Omega_x$ and $\Omega_y$ represent the deviations of the precession axis. Note that the $\mathbf{\Omega}$ depends on each state indexed by the combined wavevector and band index $\alpha$, but we skip these state indices below for brevity.

Consider the trajectory of a single electron spin on the Bloch sphere due to this precession between scattering events. We can resolve the initial spin $\hat{S}_i$ at $t = 0$ into components parallel and perpendicular to the precession axis, $\hat{S}_i^{\parallel} = (\hat{S}_i \cdot \hat{\Omega})\hat{\Omega}$ and $\hat{S}_i^{\perp} = \hat{S}_i - \hat{S}_i^{\parallel}$ respectively. The exact trajectory is then a circular motion of $\hat{S}_i^{\perp}$ in the plane perpendicular to $\hat{\Omega}$, given by

$$\hat{S}(t) = \hat{S}_i^{\parallel} + \hat{S}_i^{\perp} \cos \Omega t + \hat{\Omega} \times \hat{S}_i^{\perp} \sin \Omega t \tag{4}$$

Let $\hat{S}_i$ correspond to polar angle $\theta$ and azimuthal angle $\phi = 0$ in spherical coordinates, and expand the above for small deviations ($\hat{\Omega}_{xy}$) in the precession axis,

$$\begin{aligned} \hat{S}(t) = {} & \hat{x}(\sin\theta \cos\Omega t + \hat{\Omega}_x \cos\theta(1 - \cos\Omega t) + \hat{\Omega}_y \cos\theta \sin\Omega t) \\ & + \hat{y}(\sin\theta \sin\Omega t + \hat{\Omega}_y \cos\theta(1 - \cos\Omega t) - \hat{\Omega}_x \cos\theta \sin\Omega t) \\ & + \hat{z}(\cos\theta + \hat{\Omega}_x \sin\theta(1 - \cos\Omega t) - \hat{\Omega}_y \sin\theta \sin\Omega t) + O(\hat{\Omega}_{xy}^2). \end{aligned} \tag{5}$$

Each spin, corresponding to different wavevectors, will adopt a slightly different trajectory with the terms proportional to $\hat{\Omega}_x$ and $\hat{\Omega}_y$ vanishing in the average,

$$\langle \hat{S}(t) \rangle_{\hat{\Omega}} = \hat{x} \sin\theta \cos\bar{\Omega} t + \hat{y} \sin\theta \sin\bar{\Omega} t + \hat{z} \cos\theta, \tag{6}$$

where $\bar{\Omega} \equiv \bar{g}\mu_B B/\hbar$ is the average precession frequency. Consequently, the deviation of the spin from the average since the last scattering event at $t = 0$ is

$$\begin{aligned}\delta\hat{S}(t) = \hat{x}(\sin\theta(\cos\Omega t - \cos\bar{\Omega}t) + \hat{\Omega}_x\cos\theta(1-\cos\Omega t) + \hat{\Omega}_y\cos\theta\sin\Omega t)\\ + \hat{y}(\sin\theta(\sin\Omega t - \sin\bar{\Omega}t) + \hat{\Omega}_y\cos\theta(1-\cos\Omega t) - \hat{\Omega}_x\cos\theta\sin\Omega t)\\ + \hat{z}(\hat{\Omega}_x\sin\theta(1-\cos\Omega t) - \hat{\Omega}_y\sin\theta\sin\Omega t).\end{aligned} \tag{7}$$

The mean deviation since the large scattering event will of course be zero, by definition, but the mean-squared deviation will be non-zero. This allows us to quantify how much the spins spread out between scattering events as they random walk on the Bloch sphere, which leads to spin relaxation ($T_1$ or $T_2$ depending on the $\theta$ considered, as we specialize below). The squared deviation of the spin, separating out terms that are odd in $\hat{\Omega}_x$ and $\hat{\Omega}_y$ that will vanish upon averaging, is

$$\begin{aligned}|\delta\hat{S}(t)|^2 = 2\sin^2\theta(1-\cos(\Omega-\bar{\Omega})t)\\ + \hat{\Omega}_x^2((1-\cos\Omega t)^2 + \cos^2\theta\sin^2\Omega t)\\ + \hat{\Omega}_y^2(\cos^2\theta(1-\cos\Omega t)^2 + \sin^2\Omega t)) + O(\hat{\Omega}_x, \hat{\Omega}_y, \hat{\Omega}_x\hat{\Omega}_y).\end{aligned} \tag{8}$$

We need to average $|\delta\hat{S}(t)|^2$ over both the time since last scattering, with probability density $e^{-t/\tau_p}/\tau_p$ depending on the momentum scattering time $\tau_p$, and the variation of $\mathbf{\Omega}$ with electronic state. For the first term above, it is easier to carry out the time averaging first, while for the second term, it is easier to first average over $\hat{\Omega}$. Specifically, $\langle\hat{\Omega}_x^2\rangle_{\mathbf{\Omega}} = \langle\hat{\Omega}_y^2\rangle_{\mathbf{\Omega}} = \sigma_\perp^2/\bar{g}^2$, where $\sigma_\perp$ is the standard deviation of each off-diagonal component of the $g$-factor. With performing one of the averages for each term above,

$$\left\langle|\delta\hat{S}(t)|^2\right\rangle_{t,\mathbf{\Omega}} = \left\langle\frac{2\sin^2\theta}{1+((\Omega-\bar{\Omega})\tau_p)^{-2}}\right\rangle_{\mathbf{\Omega}} + \frac{2(1+\cos^2\theta)\sigma_\perp^2}{\bar{g}^2}(1-\langle\cos\bar{\Omega}t\rangle_t). \tag{9}$$

Finally, we can perform the remaining average for each term. For the first term, note that the precession frequency $\Omega$ has a mean of $\bar{\Omega}$ and a standard deviation $\sigma_\parallel\mu_B B/\hbar$, where $\sigma_\parallel$ is the standard deviation of the diagonal component of the $g$-tensor. We assume a normal distribution of $\Omega$ with the above mean and standard deviation in order to analytically complete the integral. Additionally, the average spin squared decays at the rate at which the spin variance grows, yielding

$$-\frac{d\bar{S}^2}{dt} = \frac{d\langle(\delta\hat{S})^2\rangle}{dt} = \frac{\langle|\delta\hat{S}(t)|^2\rangle_{t,\mathbf{\Omega}}}{\tau_p}. \tag{10}$$

Looking at the relative rate of spin decay from the above expression, this yields an inverse spin lifetime of $\langle|\delta\hat{S}(t)|^2\rangle_{t,\mathbf{\Omega}}/(2\tau_p)$. Combining this with the remaining averages performed in Eq. (9), the lifetime $T_\theta$ of spins starting at angle $\theta$ to the magnetic field $\mathbf{B}$ is given by

$$T_\theta^{-1} = \tau_{s0}^{-1} + \frac{\sin^2\theta}{\tau_p}\left(1 - \frac{\sqrt{\pi/2}}{\sigma_\parallel\mu_B B\tau_p/\hbar}\mathrm{erfcx}\frac{\sqrt{1/2}}{\sigma_\parallel\mu_B B\tau_p/\hbar}\right) + (1+\cos^2\theta)\frac{(\sigma_\perp\mu_B B/\hbar)^2\tau_p}{1+(\bar{g}\mu_B B\tau_p/\hbar)^2}, \tag{11}$$

where $\tau_{s0}$ is the zero-field spin life time due to the Elliot-Yafet mechanism that contributes an independent spin flip rate $\tau_{s0}^{-1}$, and $\mathrm{erfcx}(x) \equiv e^{x^2}\mathrm{erfc}(x)$ is the scaled complementary error function. Finally, substituting $\theta = 0$ and $\theta = \pi/2$ to get the $T_1$ and $T_2$ times for spin relaxation parallel and perpendicular to the magnetic field, we get

$$T_1^{-1} = \tau_{s0}^{-1} + \frac{2(\sigma_\perp\mu_B B/\hbar)^2\tau_p}{1+(\bar{g}\mu_B B\tau_p/\hbar)^2} \quad \text{and} \tag{12}$$

$$T_2^{-1} = \tau_{s0}^{-1} + \frac{(\sigma_\perp\mu_B B/\hbar)^2\tau_p}{1+(\bar{g}\mu_B B\tau_p/\hbar)^2} + \frac{1}{\tau_p}\left(1 - \frac{\sqrt{\pi/2}}{\sigma_\parallel\mu_B B\tau_p/\hbar}\mathrm{erfcx}\frac{\sqrt{1/2}}{\sigma_\parallel\mu_B B\tau_p/\hbar}\right), \tag{13}$$

as written in the main text.

So far we focused on the irreversible spin relaxation combining spin precession with scattering. In order to address $T_2^*$, we need to also account for reversible spin dephasing processes due to differences in precession

frequency. First, consider the purely reversible case with no scattering, for spins starting perpendicular to the magnetic field ($\theta = \pi/2$) and ignore the changes of precession axis already accounted for above, which leads to the spin trajectory $\hat{S}(t) = \hat{x}\cos\Omega t + \hat{y}\sin\Omega t = \Re[(\hat{x} - i\hat{y})e^{i\Omega t}]$. Given a probability distribution $P(\Omega)$ of precession frequencies, the average spin magnitude evolves with time as

$$|\langle\hat{S}(t)\rangle| = \left|\Re\left[(\hat{x} - i\hat{y})\int d\Omega P(\Omega)e^{i\Omega t}\right]\right| = |\tilde{P}(t)|, \tag{14}$$

where $\tilde{P}(t)$ is the Fourier transform of $P(\Omega)$. Importantly, this implies that the pure dephasing decay profile is not exponential in general and *depends on the shape* of the probability distribution of precession frequencies. Here, assuming a normal distribution is therefore inappropriate, and we use the more realistic $\Gamma_{3/2}$ distribution arising from a thermal distribution of states and a linear variation of $\Omega$ with energy near the band edge of a semiconductor. We numerically fit the Fourier transform of the $\Gamma_{3/2}$ distribution with an exponential to determine the relation between the decay time and the standard deviation of precession frequencies. Specifically, this yields $(T_2^*)^{-1} = c_0\sigma_\parallel\mu_B B/\hbar$, with constant $c_0 = 0.4414$ depending on the shape of the distribution. (For a normal distribution, $c_0 = 0.7621$, which yielded much poorer fits to the *ab initio* results.) In the presence of scattering, the reversible dephasing applies only to unscattered carriers and the above result needs to be modulated by $\tau_p$ divided by the $T_2$ contribution from $\sigma_\parallel$, resulting in

$$T_2^{-1} = \tau_{s0}^{-1} + \frac{(\sigma_\perp\mu_B B/\hbar)^2\tau_p}{1 + (\bar{g}\mu_B B\tau_p/\hbar)^2} + \left(\frac{1}{\tau_p} + c_0\sigma_\parallel\mu_B B/\hbar\right)\left(1 - \frac{\sqrt{\pi/2}}{\sigma_\parallel\mu_B B\tau_p/\hbar}\mathrm{erfcx}\frac{\sqrt{1/2}}{\sigma_\parallel\mu_B B\tau_p/\hbar}\right), \tag{15}$$

which reduces to $T_2^{-1}$ up to an $O(B^3)$ correction for small $B$ and to the no-scattering case for large $B$.

---

[1] R. Sundararaman, K. Letchworth-Weaver, K. A. Schwarz, D. Gunceler, Y. Ozhabes, and T. Arias, Jdftx: Software for joint density-functional theory, SoftwareX **6**, 278 (2017).
[2] D. R. Hamann, Optimized norm-conserving vanderbilt pseudopotentials, Phys. Rev. B **88**, 085117 (2013).
[3] J. P. Perdew, K. Burke, and M. Ernzerhof, Generalized gradient approximation made simple, Phys. Rev. Lett. **77**, 3865 (1996).
